# Supplementary material for: The Effect of People Recommenders on Echo Chambers and Polarization
Source: arXiv:2112.00626 source file (2021-12-01)
Supplement: Supplementary file 1 [file appendix.tex]

\subsection{Rewiring}

\red{In this section, we want to explore how changing basic assumptions of \PROD\ could impact the results of our analysis. 
Rewiring policy is one of the fixed dimension of our model: 
since users have a limited attention budget, each time a new connection is created another one - which already exists - is unplugged. 
As model designers, the question is "Which is the most \textit{realistic} way to select the link to exclude?". 
In order to avoid introducing any bias, we choose to select a random edge following the work by \cite{sasahara2021social}.
However, it is important to assess to which extent this design choice influences the outcomes we show in the paper. 
For this reason, we attach some experimental results obtained by adopting two additional rewiring policies: 
the first picks an edge with a probability proportional to the opinion diversity of the two nodes - the more the two opinions diverge the more is probable the edge will vanish - 
the latter aims at simulating a preferential attachment mechanism, in this case the edge is selected according to a probability inversely proportional to the degree of the node to unfollow. 
The analysis has the same setup depicted at the beginning of Section 5 with the exception that, for limited space, it is performed on two recommenders - $DJI$ and $PPR$ - 
and on four different configurations of Initial Homophily and Modularity - which represent the four angles of the heatmaps in Figure \ref{fig:nci} and \ref{fig:rwc}.
The results in Figure \ref{fig:rewiring_dji} and \ref{fig:rewiring_ppr} show qualitatively comparable outcomes between the random and the degree-based policies
 except for the $\Delta$RWC achieved when using $DJI$ recommender, under high initial homophily and high modularity. 
 The rewiring based on the opinion diversity is the most disruptive one 
 since either it greatly amplifies the polarizing effect - if it is already present - or it inverses the trend as in Figure \ref{fig:rewiring_dji}. However, this last result is expected since this policy favors the connection of like-minded individuals, hence boosting the polarization measures.
}

\begin{figure}[htp]
 \centering
 \begin{tabular}{cc}
 \hspace{-43.25mm}
 \vspace{-1.75mm}
  \includegraphics[width=.515\columnwidth]{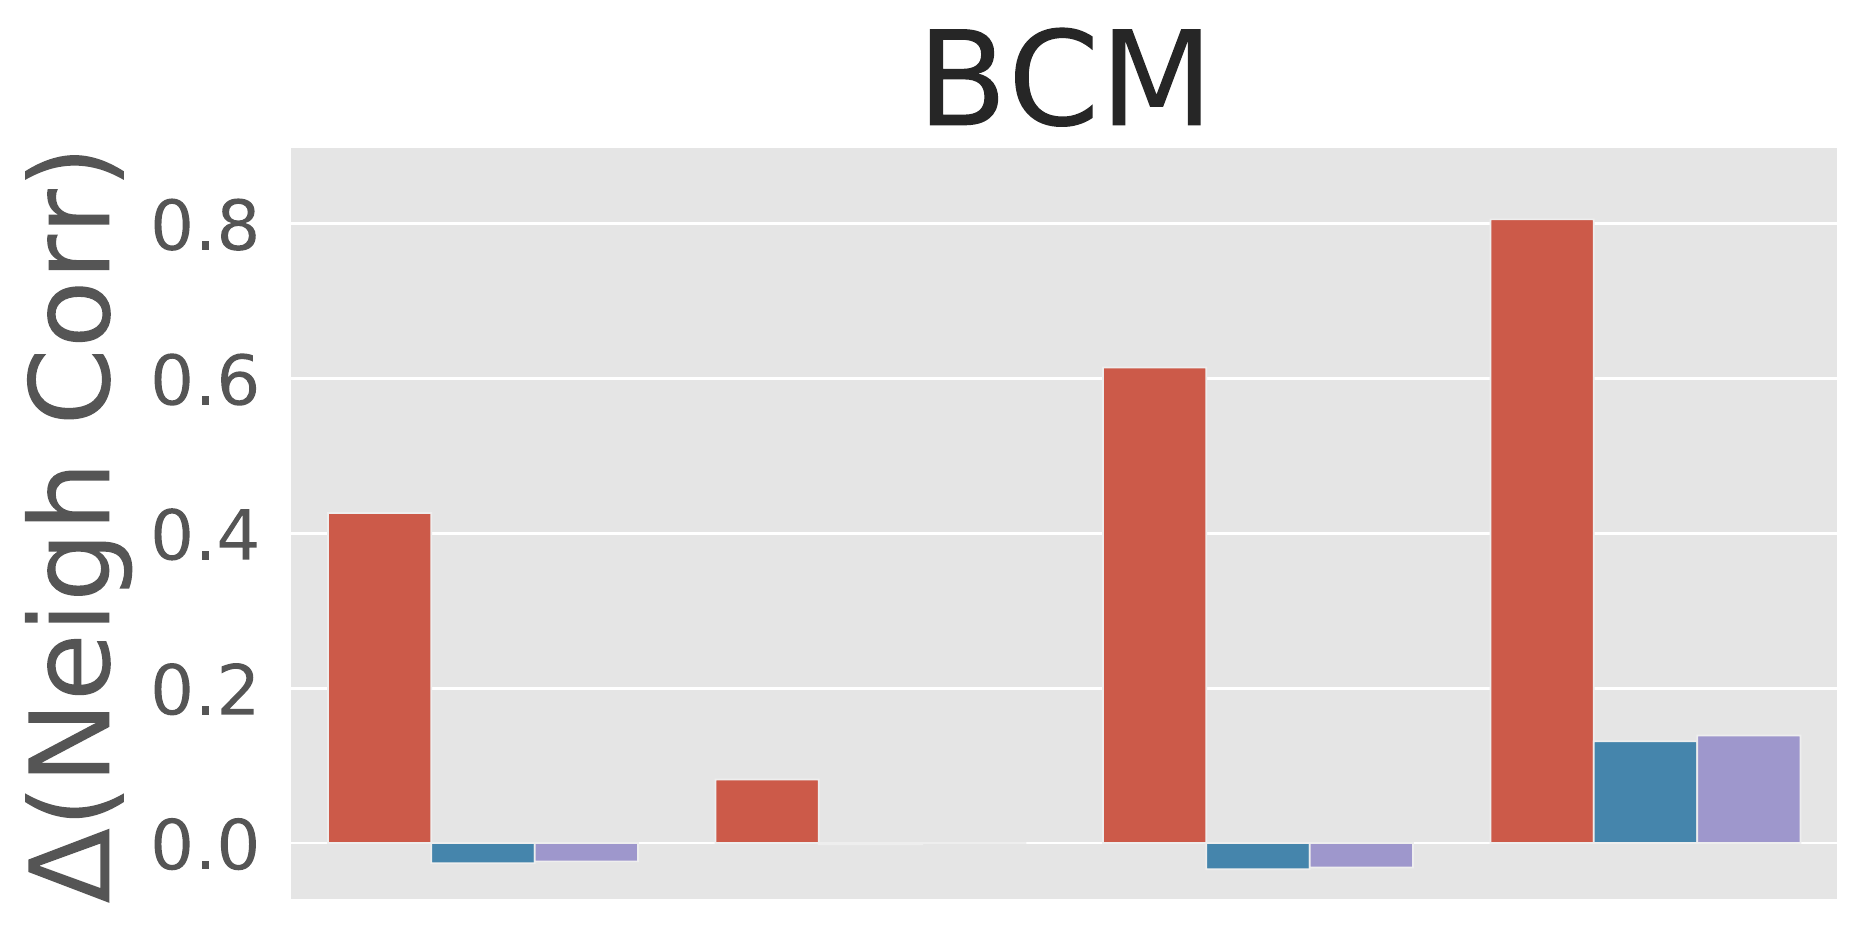}&
 \hspace{-48.25mm}
 \includegraphics[width=.5\columnwidth, height=25.65mm]{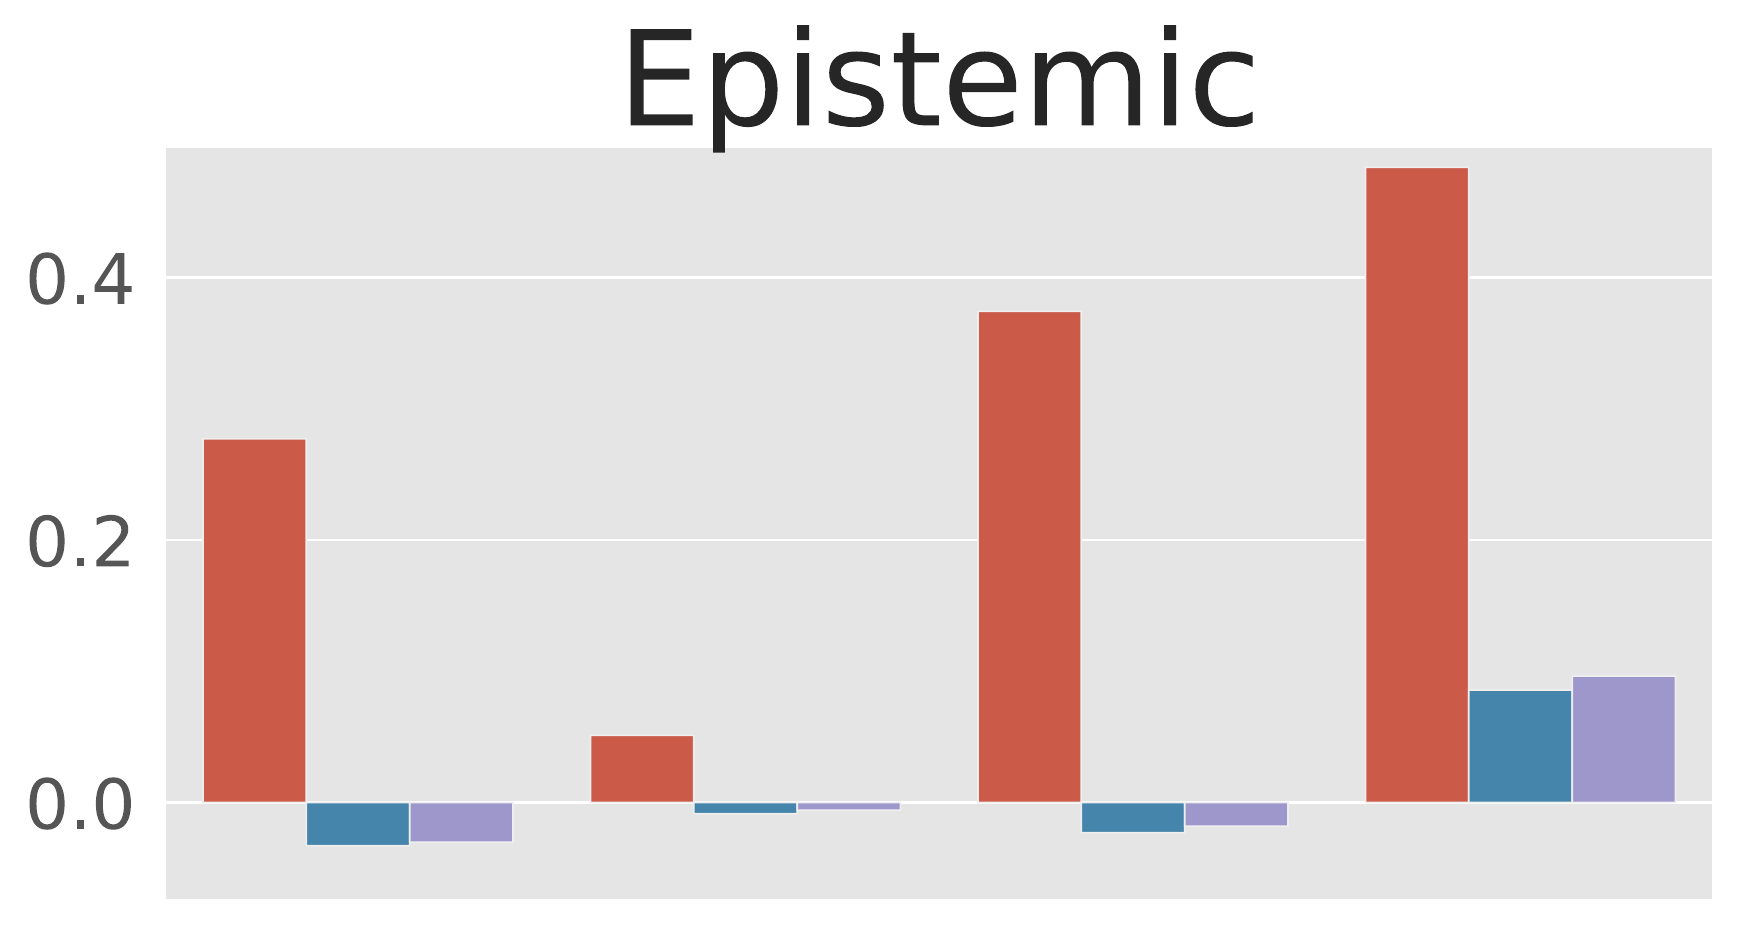} \\
 \hspace{-43.25mm}
 \includegraphics[width=.5\columnwidth, height=24.25mm]{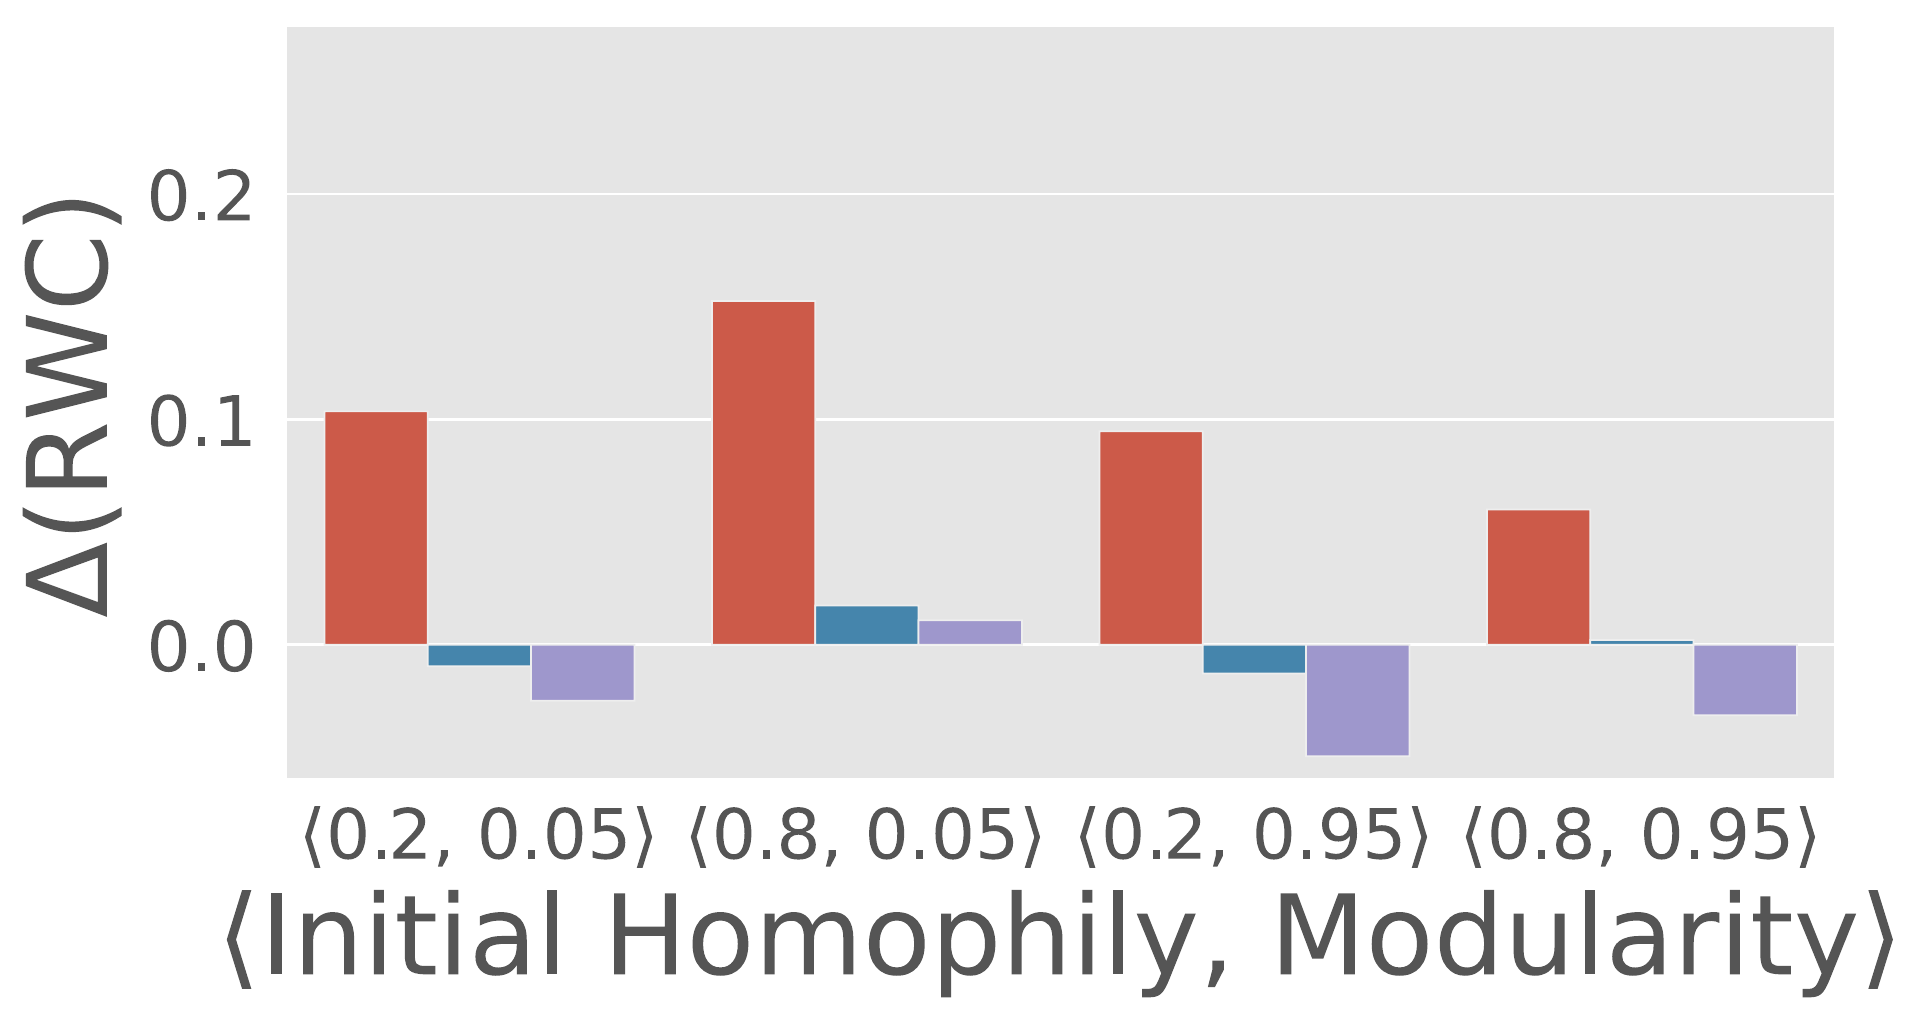}&
 \hspace{-48mm}
 \includegraphics[width=.5\columnwidth, height=25mm]{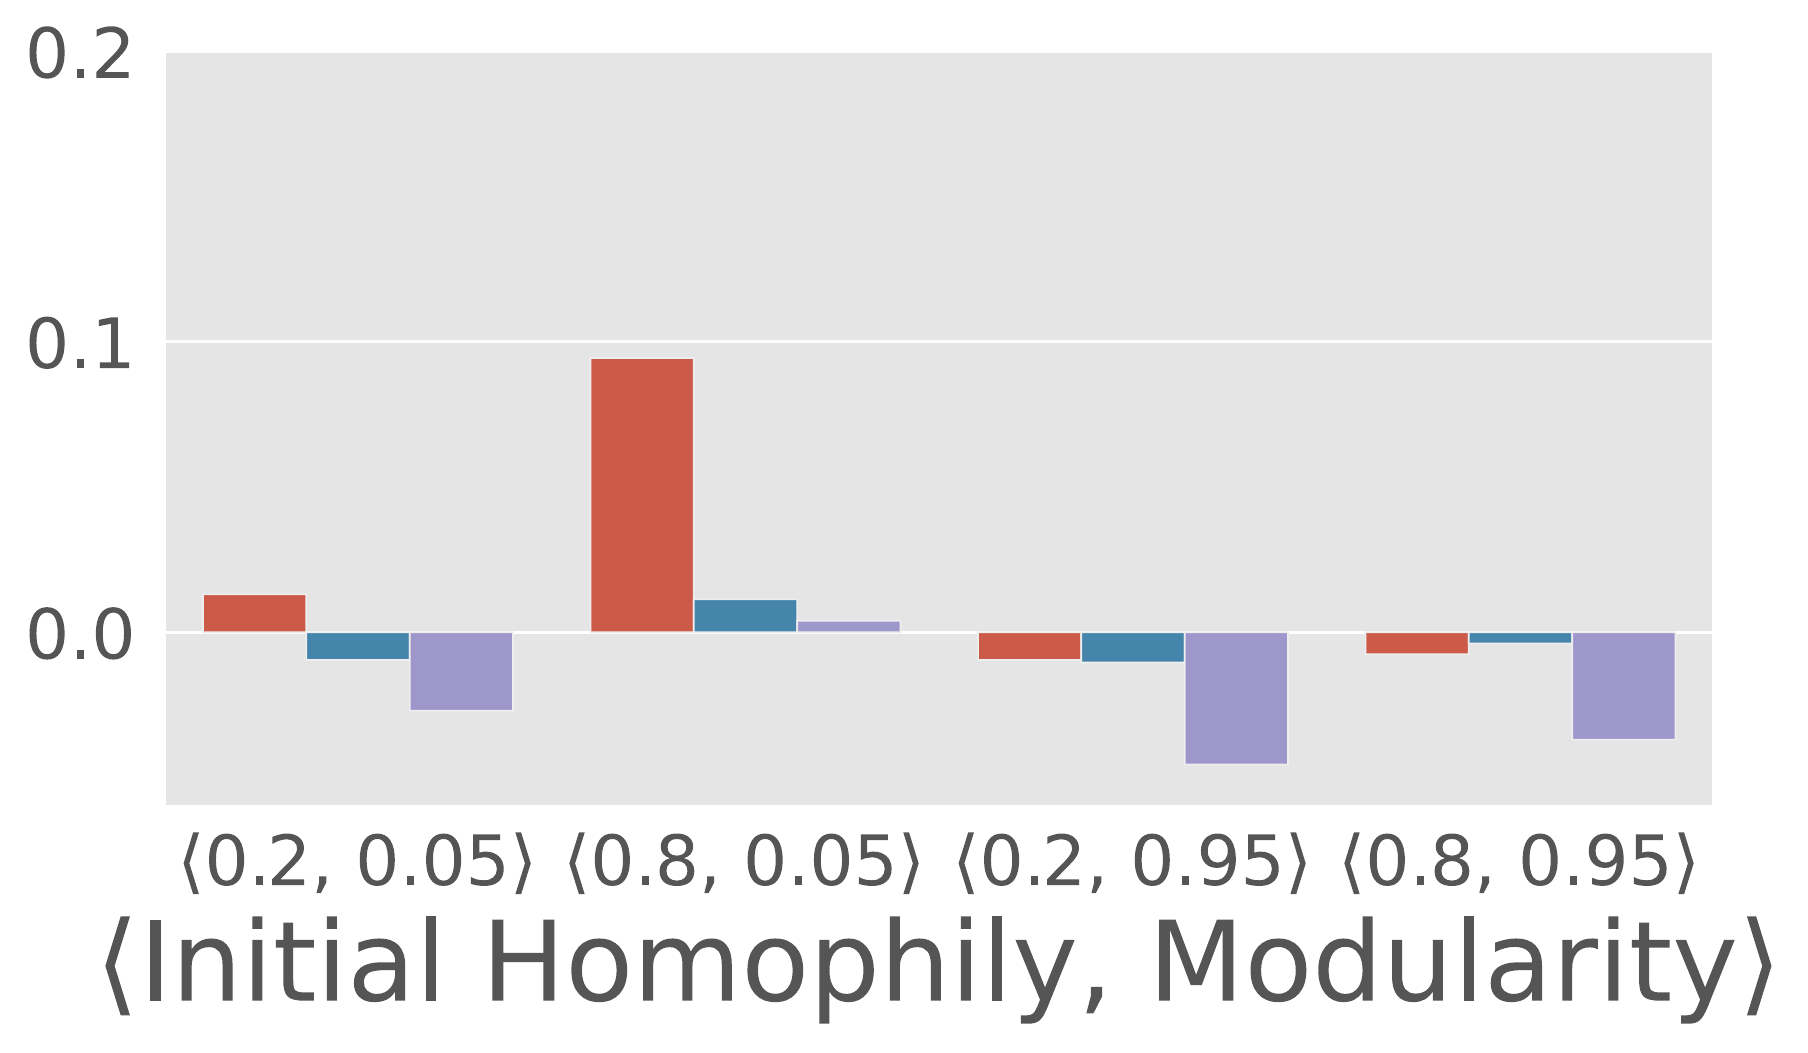} \\

  \includegraphics[width=\columnwidth]{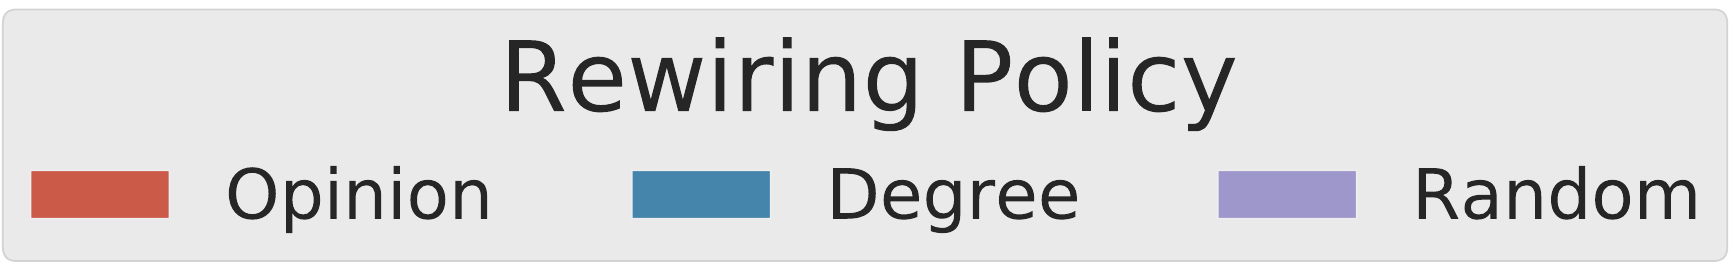}
  \hspace{-0.5mm}
 \end{tabular}
 \caption{\label{fig:rewiring_dji}
$\Delta$ NCI (first row) and $\Delta$ RWC (second row) for the BCM model (left column) and epistemological model (right column). 
Results are obtained using Directed Jaccard Index as people-recommender algorithm.
}
 \vspace{-2mm}
 \end{figure}

 \begin{figure}[htp]
 \centering
 \begin{tabular}{cc}
 \hspace{-43.25mm}
 \vspace{-1.75mm}
  \includegraphics[width=.515\columnwidth]{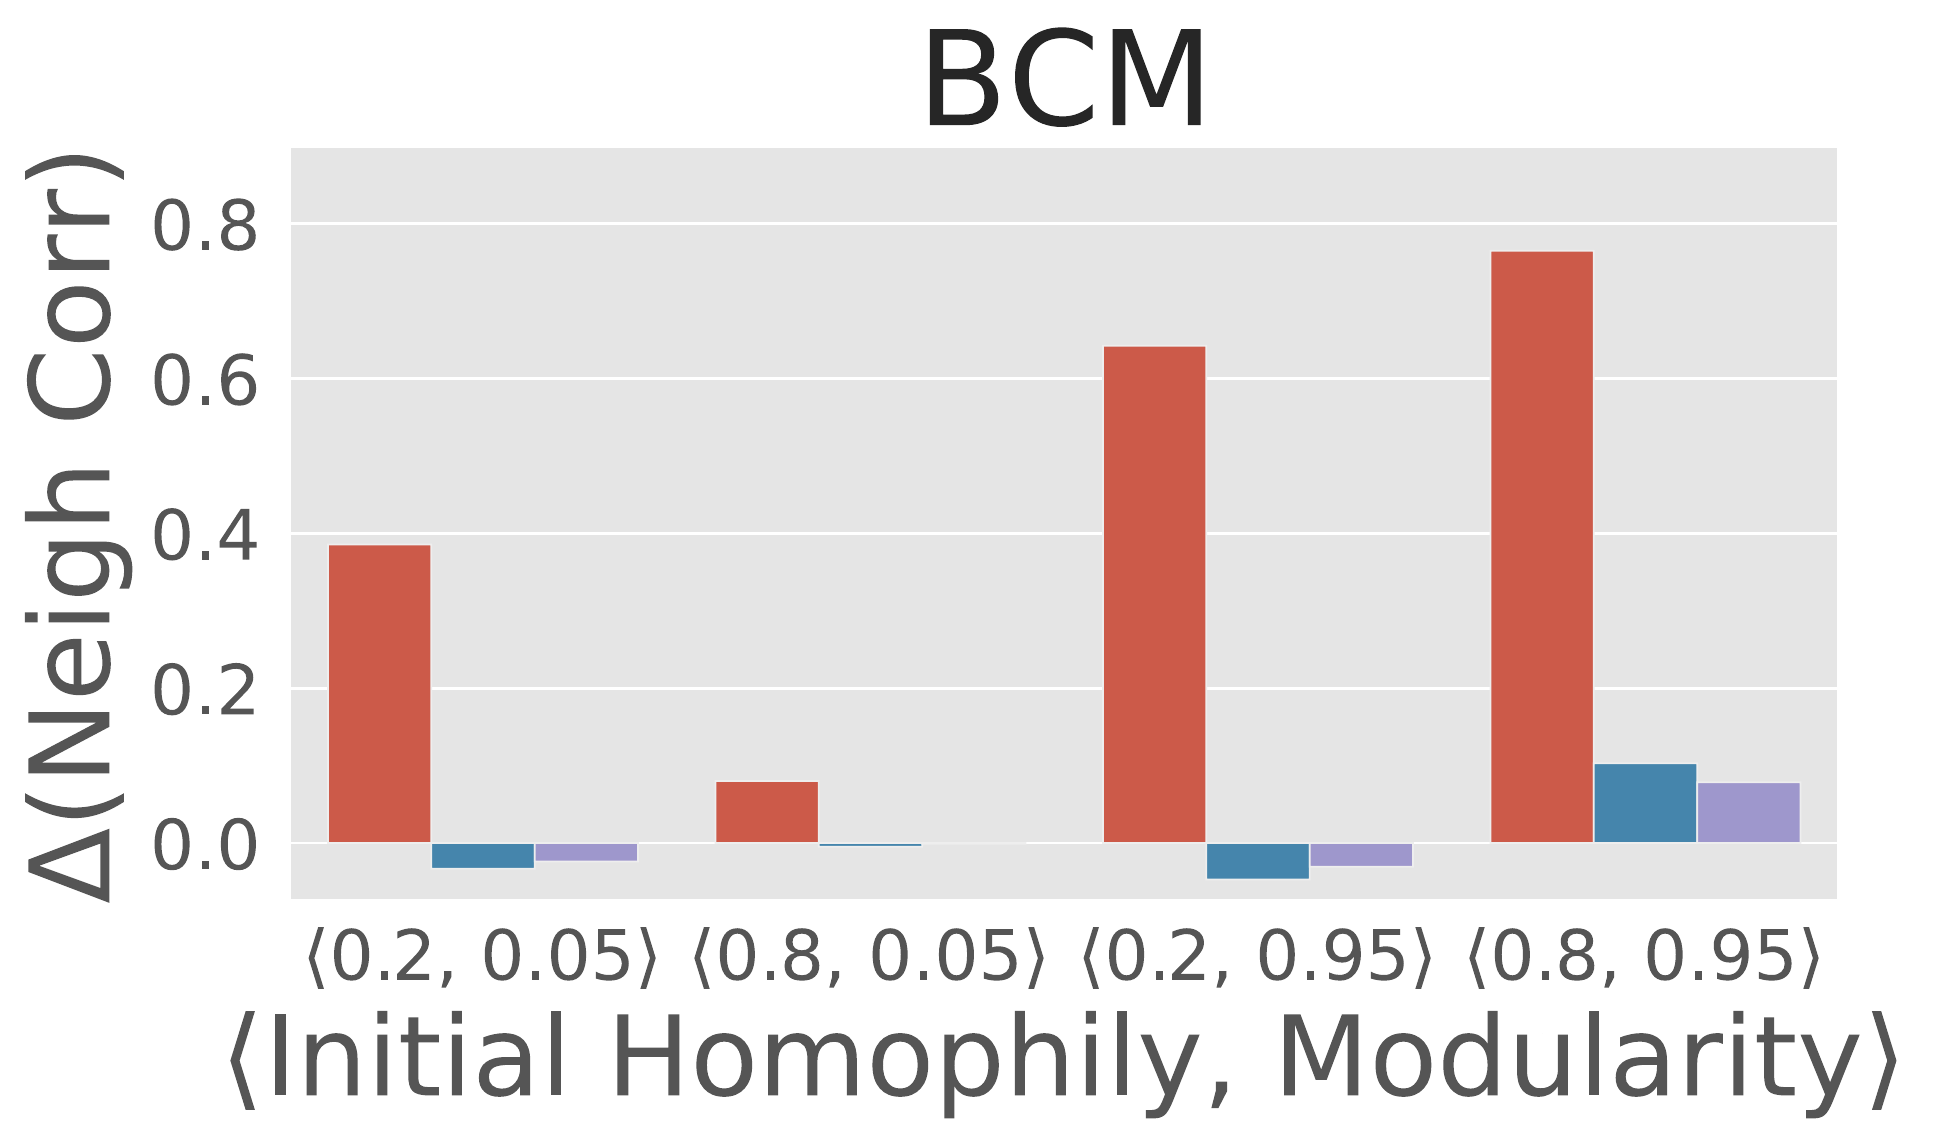}&
 \hspace{-48.25mm}
 \includegraphics[width=.5\columnwidth, height=25.65mm]{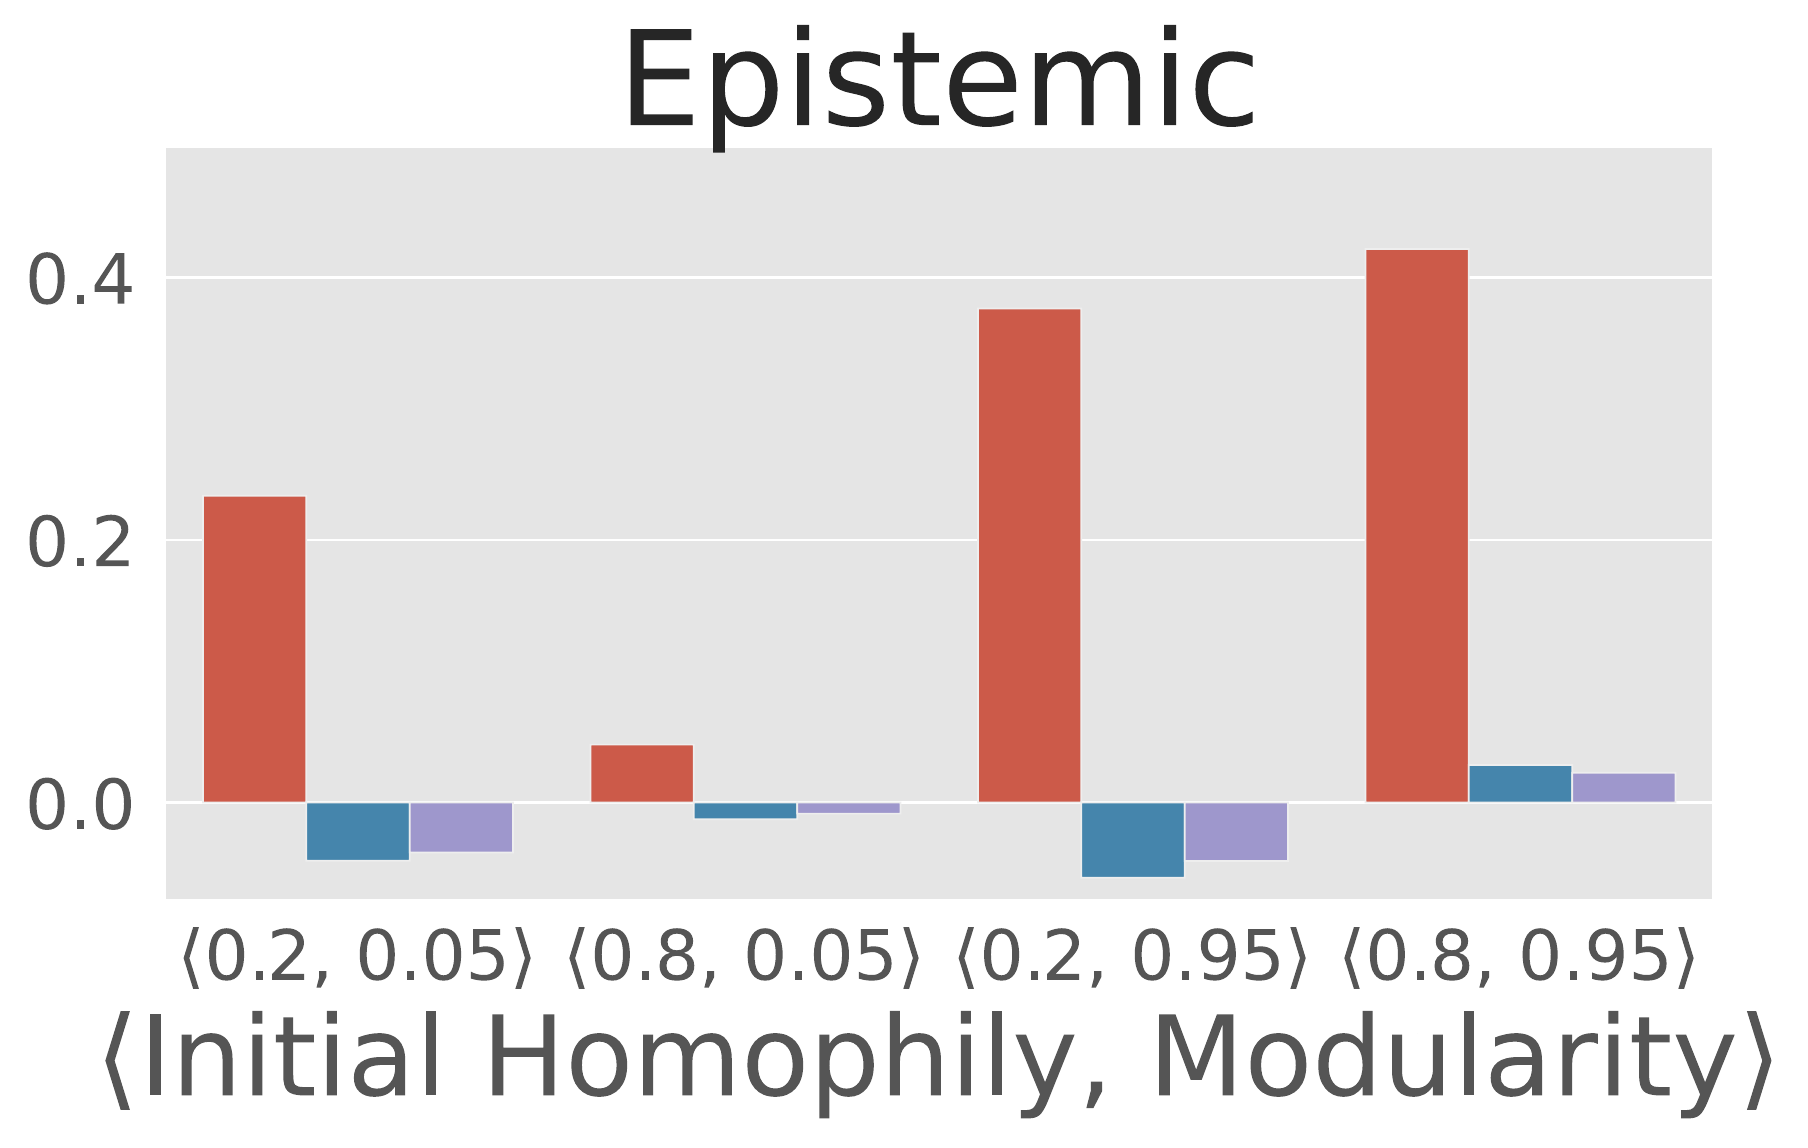} \\
 \hspace{-43.25mm}
 \includegraphics[width=.5\columnwidth, height=24.25mm]{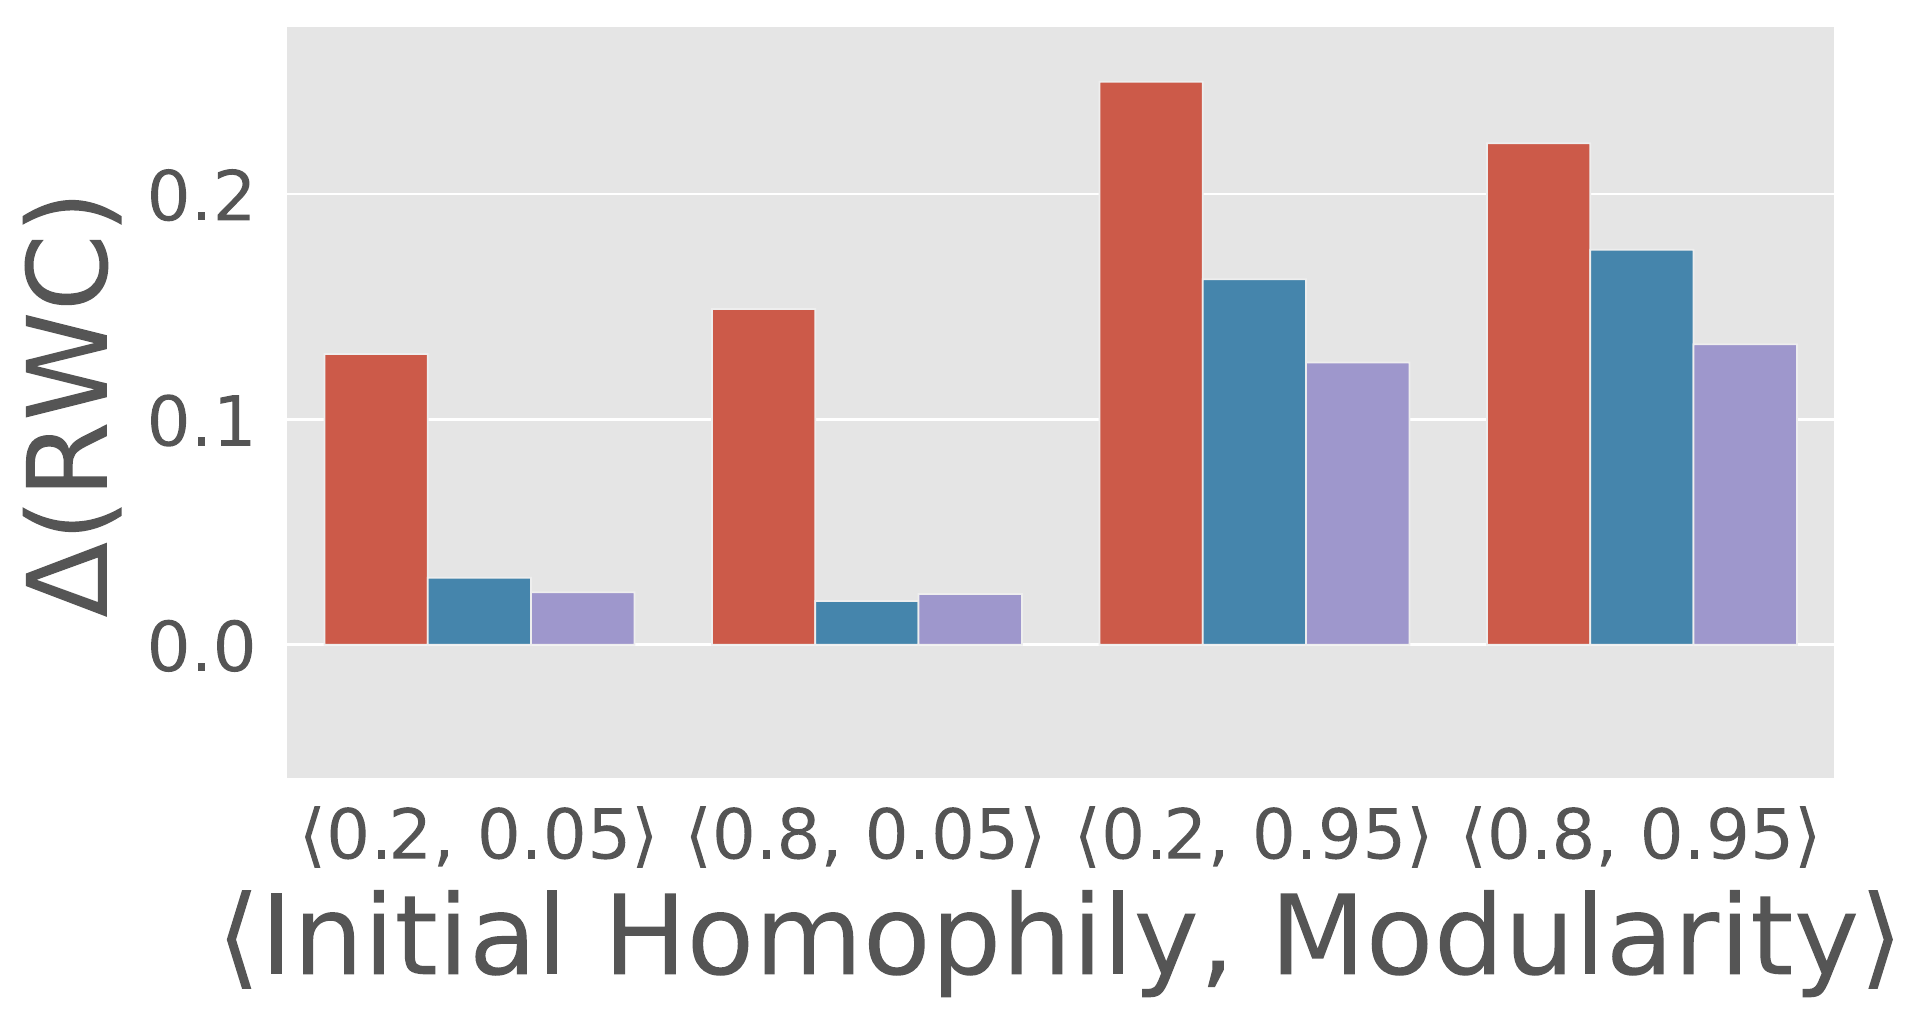}&
 \hspace{-48mm}
 \includegraphics[width=.5\columnwidth, height=25mm]{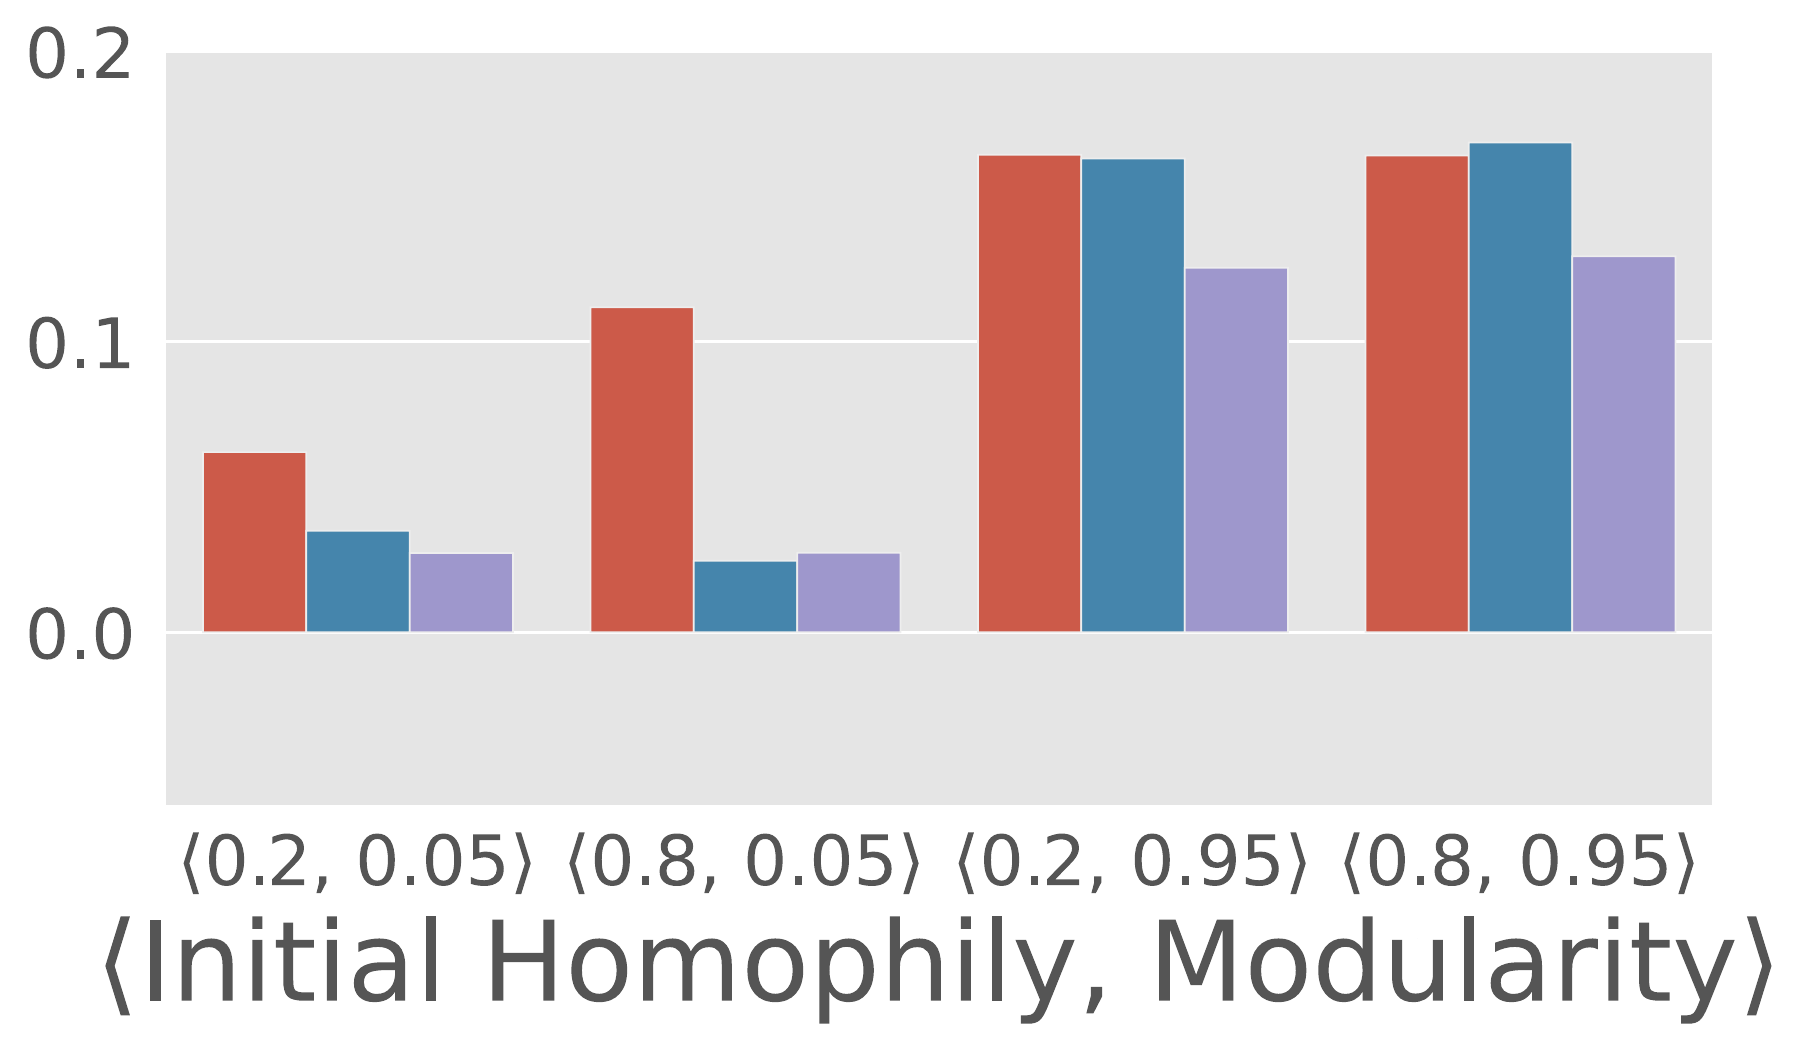} \\
 
  \includegraphics[width=\columnwidth]{rewiring_cropped_legend.pdf}
  \hspace{-0.5mm}
 \end{tabular}
 \caption{\label{fig:rewiring_ppr}
$\Delta$ NCI (first row) and $\Delta$ RWC (second row) for the BCM model (left column) and epistemological model (right column). 
Results are obtained using Personalized PageRank as people-recommender algorithm.}
 \vspace{-2mm}
 \end{figure}
